# Supplementary material for: Exceptionally strong phonon scattering by B substitution in cubic SiC
Source: arXiv:1703.04996 source file (2017-03-15)
Supplement: Supplementary file 1 [file supplementary.pdf]

# Exceptionally strong phonon scattering by B substitution in cubic SiC: Supplementary Material

Ankita Katre,[*] Jesús Carrete, Bonny Dongre, Georg K. H. Madsen, and Natalio Mingo[†]
*LITEN, CEA-Grenoble, 17 rue des Martyrs, 38054 Grenoble Cedex 9, France,*
*Institute of Materials Chemistry, TU Wien, A-1060 Vienna, Austria*

[*] ankitamkatre@gmail.com
[†] natalio.mingo@cea.fr

# I. COMPUTATIONAL DETAILS

## A. Lattice thermal conductivity

In the relaxation-time approximation, the lattice thermal conductivity $\kappa$ for isotropic compounds can be expressed as [1, 2]

$$\kappa = \frac{1}{3}\sum_j \int \frac{\mathrm{d}\mathbf{q}}{(2\pi)^3} C_{j\mathbf{q}} v_{j\mathbf{q}}^2 \tau_{j\mathbf{q}} \tag{1}$$

where $v_{j\mathbf{q}}$, $C_{j\mathbf{q}}$ and $\tau_{j\mathbf{q}}$ represent the group velocity, contribution to the specific heat, and relaxation time for phonons in mode $j\mathbf{q}$. Here, $j$ stands for the phonon branch index and $\mathbf{q}$ for the wave vector. The inverse of the phonon relaxation time, $\tau_{j\mathbf{q}}^{-1}$, is the phonon scattaring rate. This expression holds as long as none of the scattering mechanisms breaks the isotropy of the crystal. This can be true even for anisotropic defects, as long as their orientations are randomly and uniformly distributed.

## B. Total scattering rate

For the system under study in this work, the total phonon scattering rate $\tau_{j\mathbf{q}}^{-1}$ can be written as the sum of four contributions from different scattering mechanisms:

$$\tau_{j\mathbf{q}}^{-1} = \tau_{j\mathbf{q},\mathrm{anh}}^{-1} + \tau_{j\mathbf{q},\mathrm{iso}}^{-1} + \tau_{j\mathbf{q},\mathrm{def}}^{-1} + \tau_{j\mathbf{q},\mathrm{grain}}^{-1}. \tag{2}$$

where $\tau_{\mathrm{anh}}^{-1}$ is due to the intrinsic anharmonicity of the crystal that enables three-phonon processes, $\tau_{\mathrm{iso}}^{-1}$ to isotopic mass disorder, $\tau_{\mathrm{def}}^{-1}$ to crystallographic defects and $\tau_{\mathrm{grain}}^{-1}$ to the presence of grain boundaries. Anharmonic scattering is characterized using the method described in Refs. 1 and 2, based on *ab-initio* calculations of the third-order interatomic force constants (IFCs) of the perfect 3C-SiC crystal. $\tau_{\mathrm{iso}}^{-1}$ is obtained using the scheme developed by Tamura *et al.* in Refs. 3 and 4, which only requires knowledge of the phonon spectrum and the natural isotopic abundances. The expression for $\tau_{\mathrm{grain}}^{-1}$ is given in the main text. The next section is devoted to $\tau_{j\mathbf{q},\mathrm{def}}^{-1}$.

## C. Phonon scattering by defects

An expression for $\tau_{\mathrm{def}}^{-1}$ can be obtained by adding up the scattering rates due to all possible elastic phonon scattering processes $|j\mathbf{q}\rangle \rightarrow |j'\mathbf{q}'\rangle$ as [5],

$$\tau_{j\mathbf{q},\mathrm{def}}^{-1} = \pi\chi_{\mathrm{def}} \frac{\Omega}{V_{\mathrm{def}}} \frac{1}{\omega_{j\mathbf{q}}} \sum_{j'\mathbf{q}'} \left|\langle j'\mathbf{q}' \,|\, \mathbf{T} \,|\, j\mathbf{q}\rangle\right|^2 \delta\left(\omega_{j'\mathbf{q}'}^2 - \omega_{j\mathbf{q}}^2\right), \tag{3}$$

where $\chi_{\mathrm{def}}$ is the number fraction of defects, $V_{\mathrm{def}}$ the volume of a defect, $\Omega$ the volume which is used to normalize $|j\mathbf{q}\rangle$, and $\omega$ the angular frequency of phonons. The $\mathbf{T}$ matrix is given as,

$$\mathbf{T} = \left(\mathbf{I} - \mathbf{V}\mathbf{g}^{+}\right)^{-1}\mathbf{V} \tag{4}$$

where $\mathbf{g}^{+}$ is the causal Green's function for the perfect structure, $\mathbf{V}$ the perturbation matrix connecting the perfect and defective systems, and $\mathbf{I}$ the identity matrix. However, it is more convenient to dispense with the sum over outgoing phonon modes by using the optical theorem [6]:

$$\tau_{j\mathbf{q},\mathrm{def}}^{-1} = -\chi_{\mathrm{def}} \frac{\Omega}{V_{\mathrm{def}}} \frac{1}{\omega_{j\mathbf{q}}} \Im\left\{\langle j\mathbf{q} \,|\, \mathbf{T} \,|\, j\mathbf{q}\rangle\right\}. \tag{5}$$

$\mathbf{V}$ can be decomposed as a sum of contributions from the changes in mass ($\mathbf{V}_M$) and in force constants ($\mathbf{V}_K$) between the perfect and defective structures:

$$\mathbf{V} = \mathbf{V}_K + \mathbf{V}_M \tag{6}$$

More specifically, the mass term $\mathbf{V}_M$ is diagonal and its only nonzero elements correspond to onsite terms for the defect. Their values are $-\frac{M_i'-M_i}{M_i}\omega^2$, where $M'$ and $M$ are the masses of the defect and of the original atom at the $i$-th site, respectively, and $\omega$ is the angular frequency of the incoming phonon. Hence, $\mathbf{V}_M$ is independent of the structural distortions around the defect. Those effects are included in the $\mathbf{V}_K$ matrix, which is computed from the differences between the IFCs for defective ($\mathbf{K}'$) and perfect ($\mathbf{K}$) structures as $\mathbf{V}_{K,i\alpha,k\beta} = \frac{K'_{i\alpha,k\beta}-K_{i\alpha,k\beta}}{\sqrt{M_i M_k}}$. Here $i, k$ are atom indices and $\alpha, \beta$ represent Cartesian axes.

Since the perturbations are represented in real space, the need arises to impose a cutoff radius $r_{\text{cut}}$ for structural distortions. The changes in IFCs are taken into account up to second nearest-neighbours of all the atoms within this $r_{\text{cut}}$. A large $r_{\text{cut}} = 5.5$ Å (corresponding to the sixth neighbour shell in 3C-SiC) is chosen for all the defects. Changes beyond this cutoff are found to be very small. Nevertheless, it is necessary to apply a numerical correction to the "raw" $\mathbf{V}_K$ to make this cutoff strict. In particular, this ensures that all sets of IFCs fulfil the so called "sum rules" expressing the conservation of momentum or, in other words, the homogeneity of space. In practice, this is achieved by restricting $\mathbf{V}_K$ to a subspace of atomic displacements from which rigid translations have been removed. Let $\mathbf{u}_\alpha$ be the vector with component $(i, \beta)$ equal to $\delta_{\beta\alpha}$, representing a rigid displacement of all atoms along Cartesian axis $\alpha$. The restriction operator is defined as:

$$\mathbf{P} = \mathbf{I} - \sum_\alpha \mathbf{v}_\alpha \otimes \mathbf{v}_\alpha, \tag{7}$$

where $\mathbf{v}_\alpha = \mathbf{u}_\alpha / |\mathbf{u}_\alpha|$. This operator is applied on $\tilde{\mathbf{V}}_K = \mathbf{K}' - \mathbf{K}$ simply as

$$\tilde{\mathbf{V}}_K^{\text{cut}} = \mathbf{P}\tilde{\mathbf{V}}_K\mathbf{P}, \tag{8}$$

after which $\mathbf{V}_K^{\text{cut}}$ is trivially obtained from $\tilde{\mathbf{V}}_K^{\text{cut}}$. As a matter of fact, we use an iterative scheme, looping over Eq. 8 with $\tilde{\mathbf{V}}_K = \tilde{\mathbf{V}}_K^{\text{cut}}$, until the final $\mathbf{V}_K^{\text{cut}}$ components beyond the $r_{cut}$ are negligible. This ensures that no corrections to the force constants for atoms beyond $r_{cut}$ are made.

### D. Parameters for *ab-initio* calculations

The harmonic and anharmonic IFCs for 3C-SiC are calculated with a finite displacement scheme for a $5 \times 5 \times 5$ supercell of the rhombohedral primitive cell (spacegroup F-43m). The supercell contains 250 atoms. As a check, the harmonic IFCs are also obtained for a $4 \times 4 \times 4$ supercell. The maximum difference in angular frequency $\omega$ at the $\Gamma$-point is a mere 0.3 rad/ps.

All *ab-initio* calculations, including both the structural relaxation and the force calculations needed for computing the IFCs, are carried out using the projector-augmented-wave method [7] as implemented in the density functional theory package VASP [8], with the local density approximation to exchange and correlation [9]. The equilibrium lattice parameter obtained for perfect 3C-SiC is $a = 4.33$ Å.

Force constants for the $\text{B}_\text{C}$, $\text{N}_\text{C}$ and $\text{Al}_\text{Si}$ substitutional defects are calculated using $5 \times 5 \times 5$ containing one defect atom. A $4 \times 4 \times 4$ supercell is used for the carbon vacancy.

The atomic coordinates of the defective supercell are relaxed keeping the cell volume fixed before calculating the IFCs. The relaxation is iterated to avoid any imaginary phonon frequencies at the $\Gamma$-point of the Brillouin zone for the supercell. A small displacement of the defect atom or its nearest-neighbors is introduced before the start of the relaxation so as to avoid the system getting trapped in a saddle point of the energy surface.

To extract the second- and third-order IFCs from the *ab-initio* calculated forces, we use the Phonopy [10] package and our own thirdorder.py code [1] respectively.

The Born effective charges and the dielectric tensor calculated with VASP are also included to account for the non-analytical correction to the dynamical matrix for a correct reproduction of LO-TO phonon splitting in 3C-SiC [11].

To compute the defect scattering, the Green's functions are calculated on a $18 \times 18 \times 18$ grid using the tetrahedron method to integrate over the Brillouin-zone [12]. All the scattering rates are calculated on a $24 \times 24 \times 24$ $\mathbf{q}$-point mesh. The calculations of the Green's functions, the scattering rates $\tau_{\text{anh}}^{-1}$, $\tau_{\text{iso}}^{-1}$, $\tau_{\text{def}}^{-1}$, $\tau_{\text{grain}}^{-1}$ and the final $\kappa$ are performed using the almaBTE code, developed in house [13].

## II. DEFECTS AS MASS PERTURBATIONS

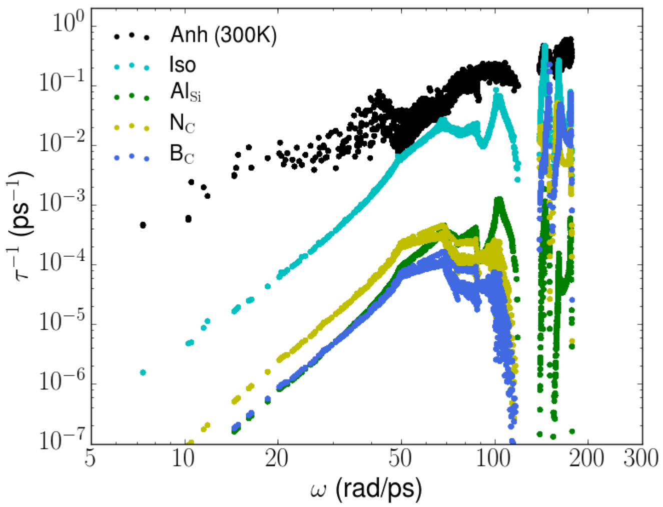


FIG. 1: Phonon scattering rates from $B_C$, $N_C$, and $Al_{Si}$ substitutional defects (in concentration of $10^{20}$ cm$^{-3}$) with only mass perturbation contributions, from isotopes and from phonon-phonon interaction at 300 K.

Fig. 1 shows the defect scattering rates from $B_C$, $N_C$, and $Al_{Si}$ taking into account only the contribution from $\mathbf{V}_M$ in Eq. (6). Slightly stronger scattering rates are obtained for the $N_C$ defect than for $B_C$ and $Al_{Si}$. However, it is clear that the contributions from all these defects are extremely weak when compared to mass-disorder and anharmonic scattering if the $\mathbf{V}_K$ term is neglected in Eq. (6).

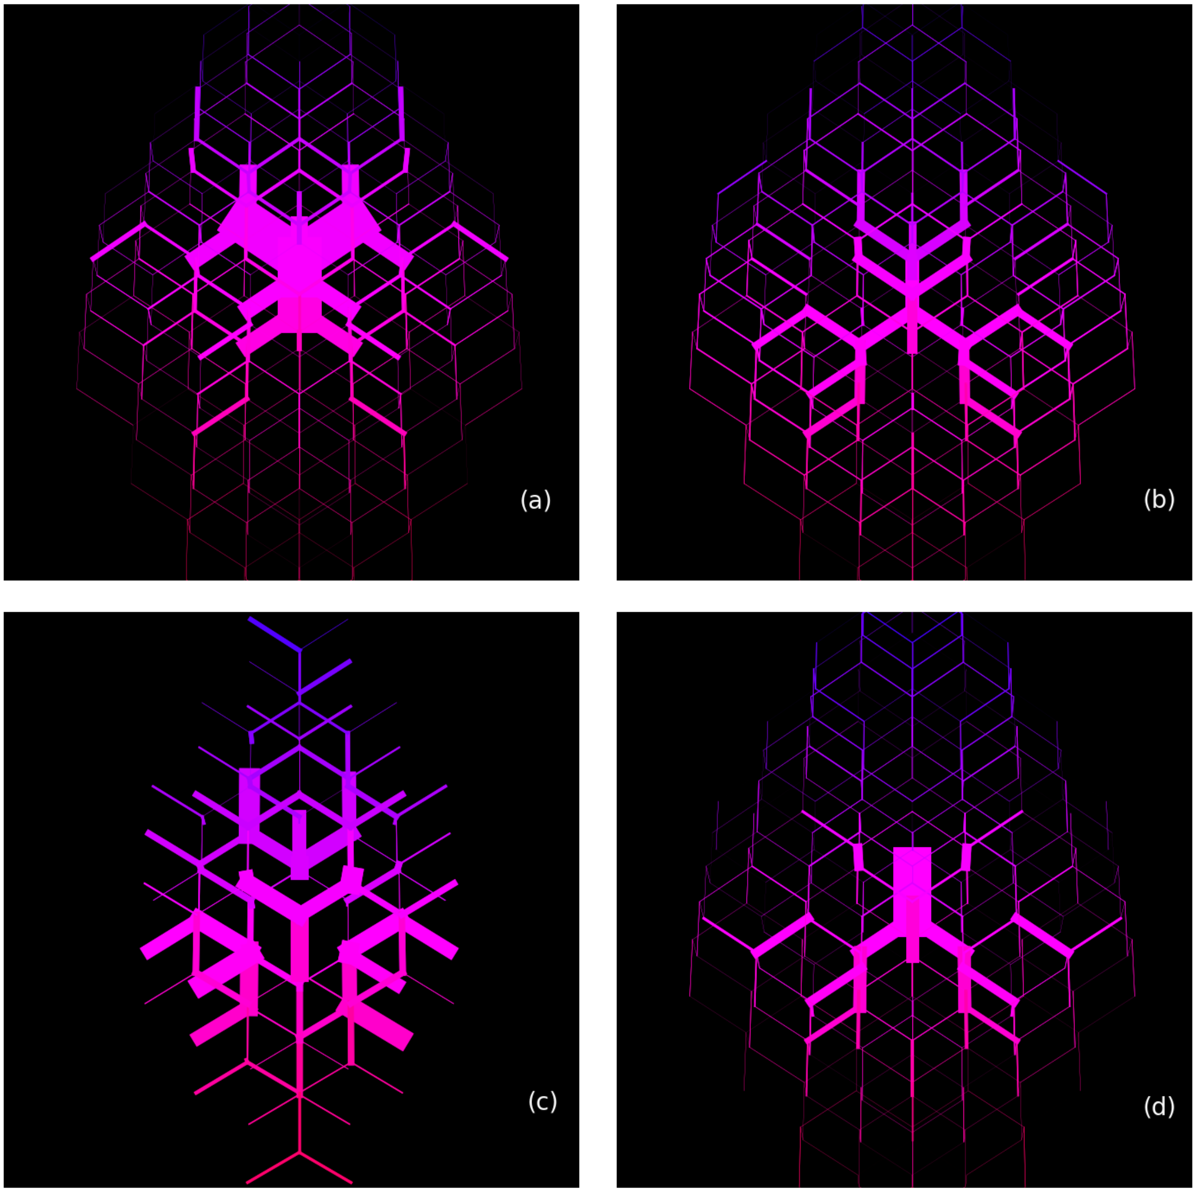


FIG. 2: Visual representation of the changes in the interatomic distances for defective supercells containing a single (a) $Al_{Si}$, (b) $N_C$, (c) $Vac_C$, or (d) $B_C$ defect in 3C-SiC. The changes in the nearest-neighbour interatomic distances are directly proportional to the bond width variations seen in the figure. The colour gradient from red to blue is used to show the depth of the bond cage structure (front to back).

## III. STRUCTURAL DISTORTION WITH DEFECTS

Fig. 2 shows a 3D representation of the bond length variations in defective 3C-SiC supercells. The defect is located in the centre of the structure. The lines represent the bonds between the nearest neighbour atoms in 3C-SiC, and their thicknesses are directly proportional to the variations in the bond lengths. Thus, lines are thicker near the defect centre and become thinner with increasing distance from the defect centre, Fig. 2. The colour gradient (red to blue) provides depth perspective to help discriminate between the bonds at the front and back in this 3D structure.

The $B_C$ defect, unlike the others, shows a surprising anisotropic behaviour of the bond length variation after the structural relaxation as seen in Fig. 2(d). Furthermore, the perturbations near the defect centre are larger than for the other two defects at C site, $N_C$ and $Vac_C$, Fig. 2(b) and (c).

[1] W. Li, J. Carrete, N. A. Katcho, and N. Mingo, Comp. Phys. Comm. **185**, 1747 (2014).
[2] A. Katre and G. K. H. Madsen, Phys. Rev. B **93**, 155203 (2016).
[3] S. Tamura, Phys. Rev. B **27**, 858 (1983).
[4] S. Tamura, Phys. Rev. B **30**, 849 (1984).
[5] N. Mingo, D. A. Stewart, D. A. Broido, L. Lindsay, and W. Li, in *Length-Scale Dependent Phonon Interactions*, edited by S. L. Shindé and G. P. Srivastava (Springer New York, 2014), no. 128 in Topics in Applied Physics, pp. 137–173, ISBN 978-1-4614-8650-3 978-1-4614-8651-0, URL `http://link.springer.com/chapter/10.1007/978-1-4614-8651-0_5`.
[6] N. Mingo, K. Esfarjani, D. A. Broido, and D. A. Stewart, Phys. Rev. B **81**, 045408 (2010).
[7] P. E. Blöchl, Phys. Rev. B **50**, 17953 (1994).
[8] G. Kresse and D. Joubert, Phys. Rev. B **59**, 1758 (1999).
[9] J. P. Perdew and A. Zunger, Phys. Rev. B **23**, 5048 (1981).
[10] A. Togo, F. Oba, and I. Tanaka, Phys. Rev. B **78**, 134106 (2008).
[11] Y. Wang, J. J. Wang, W. Y. Wang, Z. G. Mei, S. L. Shang, L. Q. Chen, and Z. K. Liu, J. Phys.: Cond. Matt. **22**, 202201 (2010).
[12] P. Lambin and J. P. Vigneron, Phys. Rev. B **29**, 3430 (1984).
[13] The ALMA project developers, *All-scale predictive design of heat management material structures*, `http://www.almabte.eu/`.
